# Supplementary material for: "There's so much responsibility on users right now:" Expert Advice for Staying Safer From Hate and Harassment
Source: arXiv:2302.08057 source file (2023-08-29)
Supplement: Supplementary file 1 [file supplementary.tex]

\section*{Supplementary Material}

\subsection{Advice Guides} \label{app:guides}

We collected 49 online support resources, filtering out those that did not address proactive practices, did not provide actionable advice, or only incidentally addressed hate and harassment, resulting in 15 guides that directly informed our list of 45 pieces of advice.

\begin{table}[h!]
\centering
\input{tables/advice_guides}
\caption{Resources we gathered advice from. }
\label{tab:advice_guides}
\end{table}

\subsection{Expert Interview Script} \label{app:script}
\setlength{\parindent}{0pt}

\textbf{Introduction}

Hi, I'm [name of primary interviewer], and I'll be leading our research session today. [Name of second interviewer] is also here to take notes and has their camera on now to say hi and so you know who else is here. \\

Thank you so much for participating in this interview.  Our goal is to understand what advice you would give Internet users to prevent or minimize their exposure to online hate and harassment. \\
So the schedule for today – I'll start by asking about your background and expertise on this topic. Then, we'll have a couple of interactive activities. And at the end, we'll have some high-level wrap-up questions. We estimate this will take about 90 minutes. Do you have a hard stop today? \\

Please keep in mind that this is not an evaluation of you or your experiences. For the purposes of this research study, there are no right or wrong answers — our goal is to learn from you and to understand your experiences and perspectives. \\

I also want to say that your participation in this study is voluntary. We are going to be talking about hate and harassment, which can be a difficult topic. You can stop or take a break at any time. If you don't want to talk about or perform any action, just let me know, and we will move on.
Any questions for me before we start? \\

And can I verify that you signed the consent form? \\

Is it okay with you if this interview is recorded? The recording will only be shared with the research team and will be deleted when the research is complete. \\

\textbf{Expert background and personal expertise}

First, I'd like to ask you about your personal expertise in this topic. What experiences or roles have you held related to the broader aim of studying or stopping online hate and harassment? \\

\textit{Follow-up questions, if not already mentioned by the participant:}
\begin{itemize}
    \item How often in your day-to-day do you advise individuals on how to stay safer from online hate and harassment?
    \item Are there any specific groups of people you have the most experience assisting (\eg activists, LGBTQ+, journalists, teens)?
    \item How long have you been working with or supporting people experiencing hate and harassment? 
    \item How did you come to this work? \\
\end{itemize}

\textbf{Threat ranking}

This first activity is about which types of hate and harassment you think the general internet user should prioritize taking action to mitigate or prevent. \\

I'm about to put a link to the tool we'll be using for the interactive activities into the chat. Please open it in your browser and present the screen with that window. Take your time, sometimes getting the permissions set up can be complicated, just let me know how it's going. \\

On the left, there are 7 categories of online hate and harassment. So the question for this activity is, for a general internet user who is not experiencing an attack right now, which threats should be their top priority for trying to mitigate or prevent? Drag the cards on the left into order in the box on the right. \\

There are no right or wrong answers here – we're just interested in your perspective of ranking these threats. To that end, please speak your thought process aloud as much as possible to help us understand what you're doing and why. \\

\textit{Follow-up questions, if not already mentioned by the participant:}
\begin{itemize}
    \item Why did you put this category at the top?
    \item How was your ranking here, for a general internet audience, informed by the population you are most familiar with? Do you think your ranking of threats would change for a different population?
    \item {[}\textit{Summarize reasons that participant mentioned.}{]} Am I correctly following how you are evaluating these threats? \\
\end{itemize}

Great, we can move on to the next activity. Click the ``Finished'' button in the upper right. \\

\textbf{Advice bucketing} [Repeat for each of the 5 parts, as described in Section~\ref{ss:procedures}]

In the next part of this interview, we have some card sorts that focus on specific, proactive advice. As you might know, there are many pieces of advice on the internet about how to stay safer from online hate and harassment. But people have limited time and energy, so it can be hard to know which advice to prioritize. \\

On the left, you’ll see a list of advice we found online for combating lockout and control. \\

We'd like you to bucket each piece of advice into high priority, medium priority, and low priority advice, or advice you don’t recommend for a general internet user. Order within the buckets doesn't matter. As before, please talk about your thought process aloud. \\

\textit{Follow-up questions, if not already mentioned by the participant:}
\begin{itemize}
    \item Why did you put this advice in the {[}high, medium, low{]} priority box?
    \item Is there any advice you feel is missing and should be added? \\
\end{itemize}

Go ahead and click ``Finished'' and we’ll move on. \\

\textbf{Specific advice: top 3}

Thanks, you can click ``Finished'', close this window and stop screensharing now. 

Now, all things considered, if you were sitting down with a general internet user, what are the top 3 pieces of advice you would give? \\

\textit{Follow-up questions, if not already mentioned by the participant:}
\begin{itemize}
    \item What makes that the most important?
    \item To the best of your knowledge, how much has this advice been adopted by general users? \\
\end{itemize}

\textbf{General thoughts}

I'm curious who the general internet user is in your mind, while you were thinking about the advice. What kind of characteristics makes for a general internet user? \\

In your own experiences helping people with online hate and harassment, how do you explain or encourage them to adopt proactive protective practices? (Or do you at all?) When are people most likely to adopt protective practices or seek help? Or if never, what barriers do they experience? When does it make the most sense for people to implement certain pieces of advice? \\

Are there any online resources or communities for general internet users about hate and harassment that you often recommend? \\

\textit{Follow-up questions, if not already mentioned by the participant:}
\begin{itemize}
    \item What makes them helpful?
    \item how easy or hard are these resources to discover before an incident occurs? How about during or after an incident? What makes it easier to discover, vs. harder?
    \item Do you think these resources are comprehensible to a wide audience? What makes them more widely accessible? Should they be?
    \item In your opinion, what, if any, are the main limitations or gaps with the resources that are currently available? \\
\end{itemize}

We've discussed a lot today about what general internet users can or should do to protect themselves from online hate and harassment. How much do you think safety currently falls on individuals right now? In the future, what would make safety less of an individual responsibility? \\

\textbf{Wrap-up}

Is there anything else you would like to say that we haven't covered? \\

Do you have any questions for me? \\

Would you like your name and/or affiliation to be acknowledged in any published material (reports, presentations) that results from this research? We will anonymize all individual responses from this interview (\eg any quotes we share from the research will not be attributed using your name or affiliation). \\

Thank you so much for your participation today - we really appreciate it! I'm going to turn off the recording now. Thank you again for sharing all your insights with us today, I hope you have a great rest of your day.
